# Supplementary material for: Next-to-leading power two-loop soft functions for the Drell-Yan process at threshold
Source: arXiv:2107.07353 ancillary file (2021-07-15)
Supplement: Supplementary file 1 [file ancillary.pdf]

July 15, 2021

# Next-to-leading power two-loop soft functions for the Drell-Yan process at threshold

ALESSANDRO BROGGIO,<sup>a,b</sup> SEBASTIAN JASKIEWICZ,<sup>c</sup> and LEONARDO VERNAZZA<sup>d,e</sup>

<sup>a</sup> *Università degli Studi di Milano-Bicocca  
Piazza della Scienza 3, I-20126 Milano, Italy*

<sup>b</sup> *INFN, Sezione di Milano-Bicocca  
Piazza della Scienza 3, I-20126 Milano, Italy*

<sup>c</sup> *Institute for Particle Physics Phenomenology, Durham University  
Durham DH1 3LE, United Kingdom*

<sup>d</sup> *Theoretical Physics Department, CERN, CH-1211 Geneva 23, Switzerland*

<sup>e</sup> *Dipartimento di Fisica Teorica, Università di Torino  
and INFN, Sezione di Torino, Via P. Giuria 1, I-10125 Torino, Italy*

## Ancillary file

In this ancillary file, we present the unintegrated squared amplitudes expressions for the real-real contributions to the generalized soft functions. The provided expressions correspond to the diagrams shown in the main text.

# 1 Squared matrix elements

## 1.1 The $S_1$ soft function

The  $S_1$  soft function is defined in Eq. (2.10). We begin with the contributions to  $S_1$  which contain a  $\delta(\omega - n_- k_1)$  constraint and are given by the sum of diagrams (a) – (g) in Figure 1. We find

$$\begin{aligned}
S_1^{(2)2r0v}(\Omega, \omega)^{\delta(\omega - n_- k_1)} &= g_s^4 \int \frac{d^d k_1}{(2\pi)^{d-1}} \int \frac{d^d k_2}{(2\pi)^{d-1}} \delta(k_1^2) \theta(k_1^0) \delta(k_2^2) \theta(k_2^0) \\
&\times \left\{ 8C_F^2 \frac{1}{(n_- k_2)} \frac{1}{(n_+ k_2)} \frac{1}{(n_- k_1)} - 2C_F C_A \frac{1}{(n_- k_2)} \frac{1}{(n_+ k_2)} \frac{1}{(n_- k_1)} \right. \\
&\quad - 2C_F C_A \frac{1}{n_+(k_1 + k_2)} \frac{1}{(n_- k_2)} \frac{1}{(n_- k_1)} \\
&\quad + C_F C_A \frac{1}{n_+(k_1 + k_2)} \frac{1}{(k_1 + k_2)^2} \frac{1}{(n_- k_1)} \frac{1}{(n_- k_2)} \left[ k_{1\perp}^2 + 2k_{2\perp} \cdot k_{1\perp} \right. \\
&\quad \left. \left. - (n_+ k_1)(n_- k_1 - n_- k_2) \right] \right. \\
&\quad + C_F C_A \frac{1}{n_-(k_1 + k_2)} \frac{1}{(k_1 + k_2)^2} \frac{1}{(n_- k_1)} \frac{1}{(n_+ k_2)} \\
&\quad \times \left[ (n_- k_1)(n_+ k_1) - (n_- k_1)(n_+ k_2) + (k_1 + k_2)^2 \right] \\
&\quad \left. + C_F C_A \frac{1}{n_+(k_1 + k_2)} \frac{1}{(k_1 + k_2)^2} \frac{1}{(n_- k_1)} \frac{1}{(n_+ k_2)} (n_+ k_1)(n_+ k_1 + 2n_+ k_2) \right\} \\
&\times \delta(\Omega - n_- k_1 - n_+ k_1 - n_- k_2 - n_+ k_2) \delta(\omega - n_- k_1). \tag{1.1}
\end{aligned}$$

Next, we have the contributions to  $S_1$  with a  $\delta(\omega - n_- k_1 - n_- k_2)$  constraint. Since only diagram (n) in Figure 1 contributes to  $C_F n_f$  piece of the cross-section, we separate the results by the colour structure. First, we have the  $C_F C_A$  proportional terms which are given by the sum of diagrams (h) – (m) in Figure 1, yielding

$$\begin{aligned}
S_1^{(2)2r0v}(\Omega, \omega)^{\delta(\omega - n_- k_1 - n_- k_2)} &= g_s^4 C_F C_A \int \frac{d^d k_1}{(2\pi)^{d-1}} \int \frac{d^d k_2}{(2\pi)^{d-1}} \delta(k_1^2) \theta(k_1^0) \delta(k_2^2) \theta(k_2^0) \\
&\times \left\{ \frac{1}{(n_-(k_1 + k_2))^2 (n_- k_1)(n_- k_2)} \left( \frac{1}{n_+ k_2} \frac{1}{n_+(k_1 + k_2)} - \frac{1}{n_+ k_1} \frac{1}{n_+(k_1 + k_2)} \right) \right. \\
&\quad \times \left[ (n_- k_1) (k_{1\perp}^2 + k_{1\perp} \cdot k_{2\perp}) - (n_- k_2) (k_{1\perp} \cdot k_{2\perp} + k_{2\perp}^2) \right] \\
&\quad \left. - \frac{1}{n_+(k_1 + k_2)} \frac{1}{n_-(k_1 + k_2)} \frac{1}{(k_1 + k_2)^2} \left( \frac{(n_- k_1 - n_- k_2)}{n_-(k_1 + k_2)(n_- k_1)(n_- k_2)} \right) \right\}
\end{aligned}$$

$$\begin{aligned}
& \times \left[ (n_- k_1) (k_{1\perp}^2 + k_{1\perp} \cdot k_{2\perp}) - (n_- k_2) (k_{1\perp} \cdot k_{2\perp} + k_{2\perp}^2) \right] \\
& + \frac{1}{n_- k_1} \left[ 2k_{1\perp}^2 + 3k_{1\perp} \cdot k_{2\perp} + k_{2\perp}^2 \right] + \frac{1}{n_- k_2} \left[ k_{1\perp}^2 + 3k_{1\perp} \cdot k_{2\perp} + 2k_{2\perp}^2 \right] \Bigg) \\
& + \frac{1}{n_- k_1} \frac{1}{n_+ k_2} \frac{1}{n_- (k_1 + k_2)} \frac{1}{(k_1 + k_2)^2} \left[ (k_{1\perp}^2 - k_{2\perp}^2) - \frac{n_- (2k_1 + k_2)}{n_- (k_1 + k_2)} (k_{1\perp} + k_{2\perp})^2 \right] \\
& - \frac{1}{n_+ (k_1 + k_2)} \frac{1}{n_+ k_2} \frac{1}{(n_- (k_1 + k_2))^2} \frac{1}{(k_1 + k_2)^2} n_+ (k_1 - k_2) (k_{1\perp} + k_{2\perp})^2 \\
& - \frac{1}{n_+ (k_1 + k_2)} \frac{1}{(k_1 + k_2)^4} n_+ k_2 \left( \frac{(k_{1\perp}^2 + k_{1\perp} \cdot k_{2\perp})}{n_- (k_1 + k_2)} - n_- k_1 \frac{(k_{1\perp} + k_{2\perp})^2}{(n_- (k_1 + k_2))^2} \right) \\
& - \frac{1}{2} \frac{1}{n_+ (k_1 + k_2)} \frac{1}{(k_1 + k_2)^4} \frac{1}{(n_- (k_1 + k_2))^2} \left( (k_{1\perp} + k_{2\perp})^2 \left[ n_- (2k_1 + k_2) n_+ (k_1 + 2k_2) \right. \right. \\
& \quad \left. \left. + n_+ (k_1 - k_2) n_- (k_1 - k_2) + n_- (k_1 + 2k_2) n_+ (2k_1 + k_2) - 8(k_1 + k_2)^2 \right] \right. \\
& \quad \left. - n_- (k_1 + k_2) n_+ (k_1 + 2k_2) (k_{1\perp}^2 + 3k_{1\perp} \cdot k_{2\perp} + 2k_{2\perp}^2) \right. \\
& \quad \left. - n_- (k_1 + k_2) n_+ (2k_1 + k_2) (2k_{1\perp}^2 + 3k_{1\perp} \cdot k_{2\perp} + k_{2\perp}^2) \right. \\
& \quad \left. + (1 - d) n_+ (k_1 - k_2) \left[ n_- (k_1 - k_2) (k_{1\perp} + k_{2\perp})^2 - n_- (k_1 + k_2) (k_{1\perp}^2 - k_{2\perp}^2) \right] \right) \Bigg\} \\
& \times \delta(\Omega - n_- k_1 - n_+ k_1 - n_- k_2 - n_+ k_2) \delta(\omega - n_- k_1 - n_- k_2). \tag{1.2}
\end{aligned}$$

Lastly for  $S_1$ , we give the contribution of the diagram in panel (n) of Figure 1, it takes the following form

$$\begin{aligned}
S_1^{(2)2r0v}(\Omega, \omega)^{fig:1(n)} &= 2g_s^4 C_F n_f \int \frac{d^d k_1}{(2\pi)^{d-1}} \int \frac{d^d k_2}{(2\pi)^{d-1}} \delta(k_1^2) \theta(k_1^0) \delta(k_2^2) \theta(k_2^0) \\
& \times \frac{1}{n_+ (k_1 + k_2)} \frac{1}{(k_1 + k_2)^4} \frac{1}{(n_- (k_1 + k_2))^2} \left( (n_- k_1) (n_+ k_2) (k_{1\perp} + k_{2\perp})^2 \right. \\
& \quad \left. - n_- (k_1 + k_2) (n_+ k_2) (k_{1\perp}^2 + k_{1\perp} \cdot k_{2\perp}) - 2k_1 \cdot k_2 (k_{1\perp} + k_{2\perp})^2 \right. \\
& \quad \left. + (n_+ k_1) (n_- k_2) (k_{1\perp} + k_{2\perp})^2 - n_- (k_1 + k_2) (n_+ k_1) (k_{1\perp} \cdot k_{2\perp} + k_{2\perp}^2) \right) \\
& \times \delta(\Omega - n_- k_1 - n_+ k_1 - n_- k_2 - n_+ k_2) \delta(\omega - n_- k_1 - n_- k_2). \tag{1.3}
\end{aligned}$$

## 1.2 The $S_3$ soft function

Next, we give the expression for the  $S_3$  soft function in (2.12). Both of the emissions occur from position  $z_-$  before crossing the cut and being absorbed by the LP conjugate amplitude, hence the  $\delta(\omega - n_-k_1 - n_-k_2)$  constraint. We find

$$\begin{aligned}
S_3^{(2)}(\Omega, \omega) = & g_s^4 C_F C_A \int \frac{d^d k_1}{(2\pi)^{d-1}} \int \frac{d^d k_2}{(2\pi)^{d-1}} \delta(k_1^2) \theta(k_1^0) \delta(k_2^2) \theta(k_2^0) \\
& \times \left\{ \frac{k_{1\perp} \cdot k_{2\perp}}{(n_-(k_1 + k_2))^2} \left( \frac{1}{n_+ k_2} \frac{1}{n_+(k_1 + k_2)} - \frac{1}{n_+ k_1} \frac{1}{n_+(k_1 + k_2)} \right) \left( \frac{1}{n_- k_1} - \frac{1}{n_- k_2} \right) \right. \\
& + \frac{1}{2} (d-2) \frac{1}{(n_-(k_1 + k_2))^3} \frac{1}{(k_1 + k_2)^2} (n_-(k_1 - k_2))^2 \\
& - \frac{1}{n_+(k_1 + k_2)} \frac{1}{(n_-(k_1 + k_2))^2} \frac{1}{(k_1 + k_2)^2} \left( \frac{1}{2} (d-2) n_+(k_1 - k_2) n_-(k_1 - k_2) \right. \\
& \quad \left. + k_{1\perp} \cdot k_{2\perp} (n_- k_1 - n_- k_2) \left( \frac{1}{n_- k_1} - \frac{1}{n_- k_2} \right) + 2k_{1\perp}^2 + 2k_{1\perp} \cdot k_{2\perp} + 2k_{2\perp}^2 \right. \\
& \quad \left. \left. - \frac{n_- k_2}{n_- k_1} (2k_{1\perp}^2 + k_{1\perp} \cdot k_{2\perp}) - \frac{n_- k_1}{n_- k_2} (2k_{2\perp}^2 + k_{1\perp} \cdot k_{2\perp}) \right) \right\} \\
& \times \delta(\Omega - n_- k_1 - n_+ k_1 - n_- k_2 - n_+ k_2) \delta(\omega - n_- k_1 - n_- k_2). \tag{1.4}
\end{aligned}$$

## 1.3 The $S_4$ soft function

For  $S_4$  soft function in Eq. (2.13) after the redefinition in (2.18) we have

$$\begin{aligned}
S_4^{(2)}(\Omega, \omega_1, \omega_2) = & g_s^4 C_F C_A \int \frac{d^d k_1}{(2\pi)^{d-1}} \int \frac{d^d k_2}{(2\pi)^{d-1}} \delta(k_1^2) \theta(k_1^0) \delta(k_2^2) \theta(k_2^0) \\
& \times \left\{ (d-2) \frac{1}{(k_1 + k_2)^2} \frac{1}{(n_-(k_1 + k_2))^3} (n_- k_2) n_-(k_1 - k_2) \right. \\
& - \frac{1}{n_+(k_1 + k_2)} \frac{1}{(k_1 + k_2)^2} \frac{1}{(n_-(k_1 + k_2))^2} \frac{1}{(n_- k_1)} \\
& \quad \times \left( 2n_-(k_2 - k_1) k_{1\perp} \cdot k_{2\perp} + 2(2k_{1\perp}^2 + k_{1\perp} \cdot k_{2\perp}) (n_- k_2) \right. \\
& \quad \left. \left. + (d-2) n_- k_2 n_- k_1 n_+(k_1 - k_2) - 2(2k_{2\perp}^2 + k_{1\perp} \cdot k_{2\perp}) (n_- k_1) \right) \right\} \\
& \times \delta(\Omega - n_- k_1 - n_+ k_1 - n_- k_2 - n_+ k_2) \delta(\omega - n_- k_1) \delta(\omega - n_- k_2). \tag{1.5}
\end{aligned}$$

## 1.4 The $S_5$ soft function

The  $S_5$  soft function, as defined in Sec. 2, is obtained by evaluating

$$\begin{aligned}
S_5^{(2)}(\Omega, \omega_1, \omega_2) &= g_s^4 \left( C_F^2 - \frac{1}{2} C_F C_A \right) \int \frac{d^d k_1}{(2\pi)^{d-1}} \int \frac{d^d k_2}{(2\pi)^{d-1}} \delta(k_1^2) \theta(k_1^0) \delta(k_2^2) \theta(k_2^0) \\
&\times 2(2 - 2\epsilon) \frac{1}{(k_1 + k_2)^2} \left( \frac{1}{n_+(k_1 + k_2)} \frac{1}{n_-(k_1 + k_2)} \frac{k_{1\perp} \cdot k_{2\perp}}{n_- k_1} + \frac{(n_- k_2)}{(n_-(k_1 + k_2))^2} \right) \\
&\times \delta(\Omega - n_- k_1 - n_+ k_1 - n_- k_2 - n_+ k_2) \delta(\omega_1 - n_- k_1) \delta(\omega_2 - n_- k_2). \quad (1.6)
\end{aligned}$$
